# Supplementary material for: Connected but Late: Sample Age of Commercial BLE Wearables under Wi-Fi Coexistence for Real-Time Clinical Applications
Source: arXiv:2611.30774 source file (2026-11-23)
Supplement: Supplementary file 1 [file supplabels.tex]

\makeatletter
\@namedef{r@S-sup:platform}{{S1}{1}{}{}{}}
\@namedef{r@S-fig:s-architecture}{{S1}{1}{}{}{}}
\@namedef{r@S-tab:s-roles}{{S1}{1}{}{}{}}
\@namedef{r@S-sup:streaming}{{S1-D}{1}{}{}{}}
\@namedef{r@S-sup:chamber}{{S2}{1}{}{}{}}
\@namedef{r@S-tab:s-ledger}{{S2}{2}{}{}{}}
\@namedef{r@S-sup:instruments}{{S2-A}{2}{}{}{}}
\@namedef{r@S-fig:s-maps}{{S2}{2}{}{}{}}
\@namedef{r@S-tab:s-conditions}{{S3}{3}{}{}{}}
\@namedef{r@S-tab:s-link}{{S4}{3}{}{}{}}
\@namedef{r@S-tab:s-zeroheadroom}{{S5}{3}{}{}{}}
\@namedef{r@S-sup:sensitivity}{{S2-F}{3}{}{}{}}
\@namedef{r@S-tab:s-sensitivity}{{S6}{4}{}{}{}}
\@namedef{r@S-sup:gym}{{S3}{4}{}{}{}}
\@namedef{r@S-fig:s-perrun}{{S3}{4}{}{}{}}
\@namedef{r@S-sup:replay}{{S4}{4}{}{}{}}
\@namedef{r@S-fig:s-load}{{S4}{5}{}{}{}}
\@namedef{r@S-tab:s-replay-steps}{{S7}{5}{}{}{}}
\@namedef{r@S-tab:s-replay-window}{{S8}{5}{}{}{}}
\@namedef{r@S-sup:benchmark}{{S5}{5}{}{}{}}
\makeatother
